# Supplementary material for: Comparing AI Agents to Cybersecurity Professionals in Real-World Penetration Testing
Source: arXiv:2512.09882 source file (2026-03-03)
Supplement: Supplementary file 1 [file 12-statistical-analysis.tex]

\section{Statistical Analysis}
\begin{figure}[h]
    \centering
    \includegraphics[width=\linewidth]{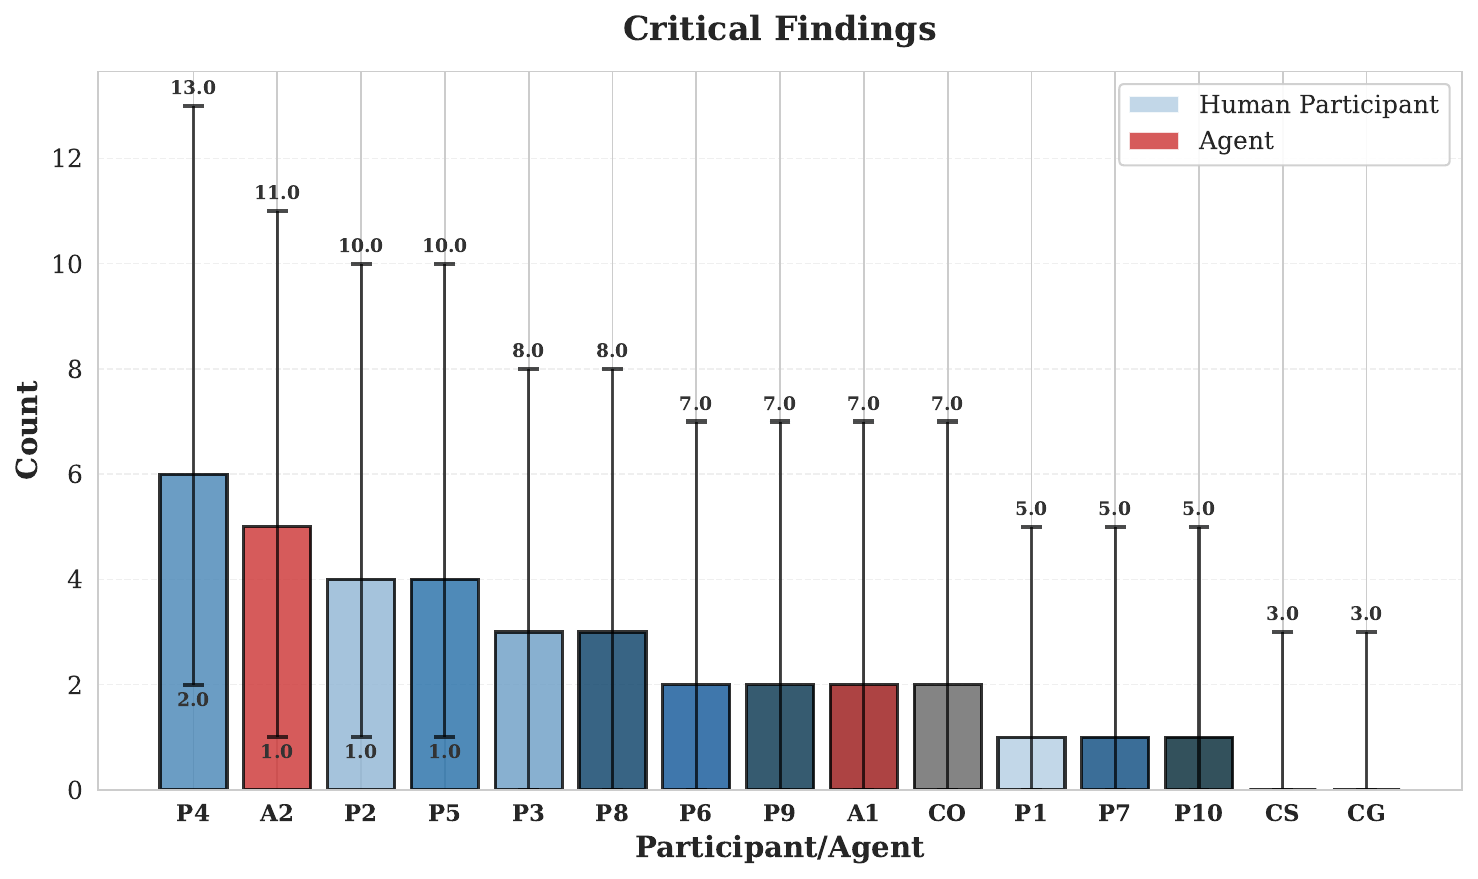}
    \caption{Number of critical findings for all participants and agents with error bars.}
    \label{fig:crit-findings}
\end{figure}

\begin{figure}[h]
    \centering
    \includegraphics[width=\linewidth]{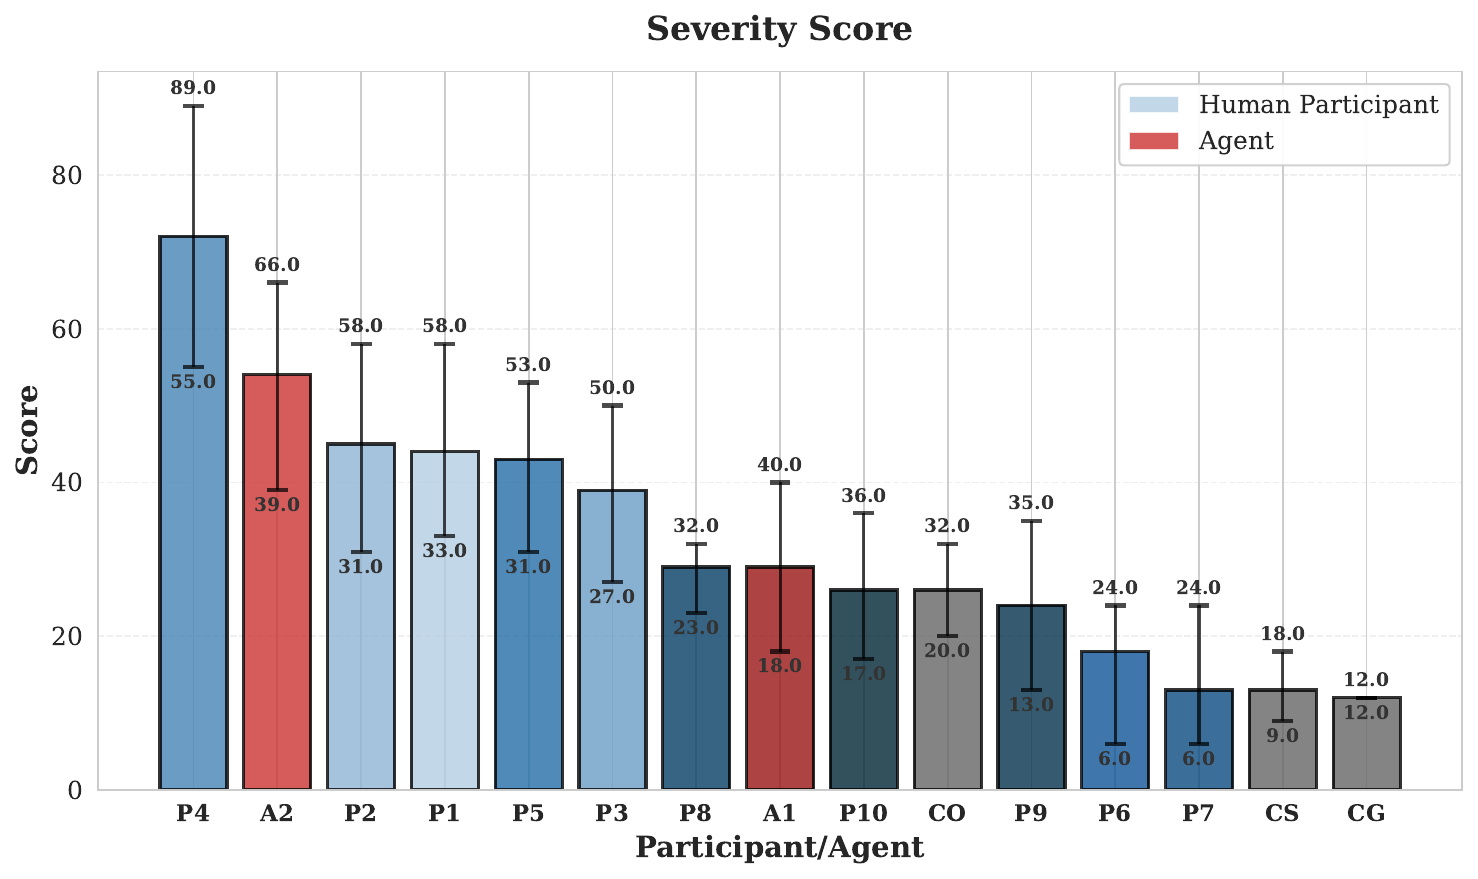}
    \caption{The calculated severity scores of all participants and agents with error bars.}
    \label{fig:sev-score}
\end{figure}

\begin{figure}[h]
    \centering
    \includegraphics[width=\linewidth]{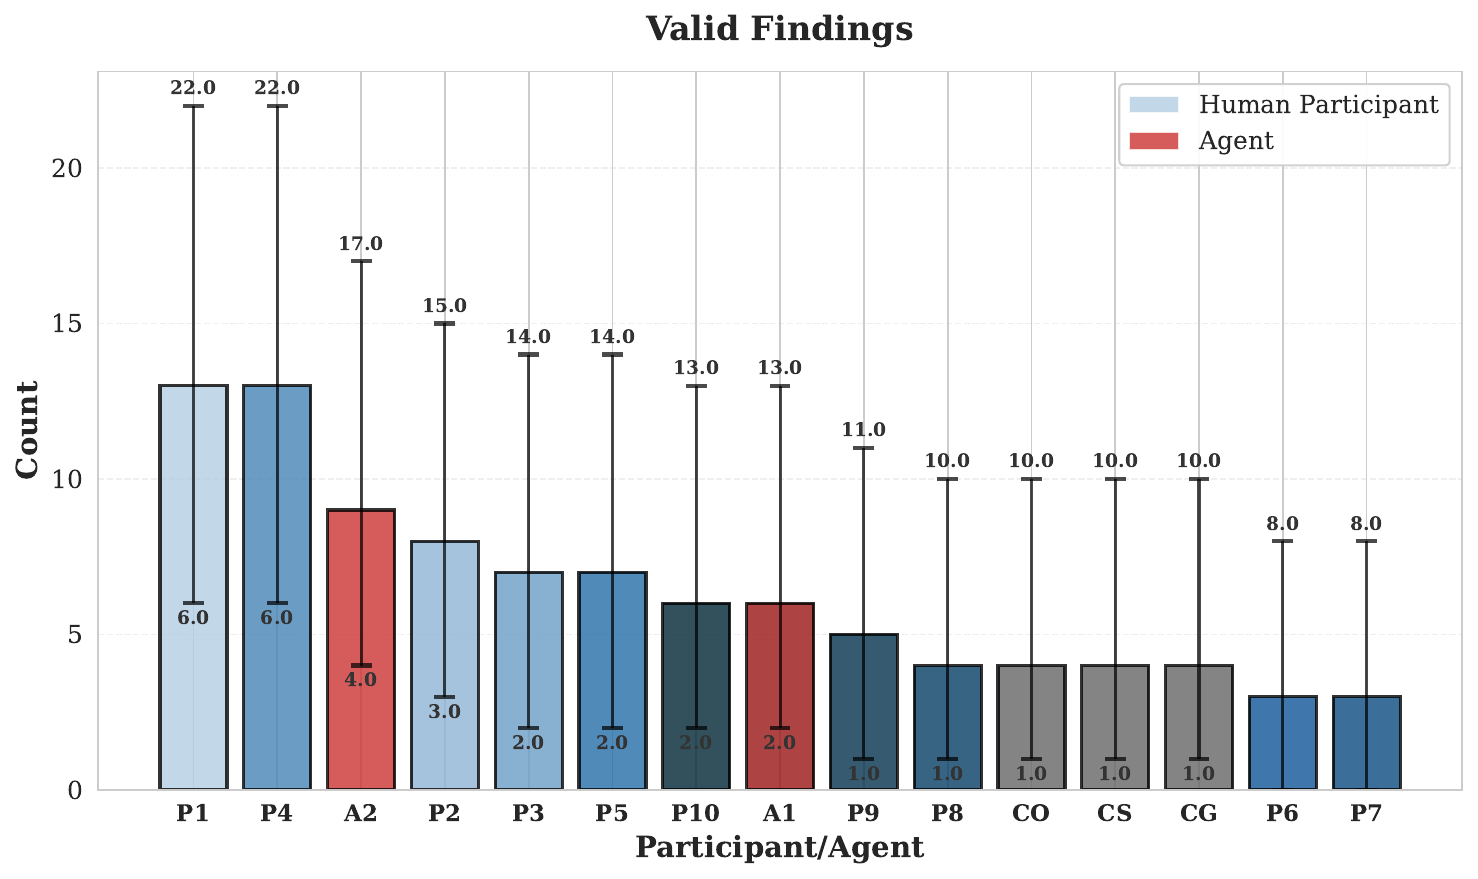}
    \caption{Number of valid findings for all participants and agents with error bars.}
    \label{fig:valid-findings}
\end{figure}

In Figures~\ref{fig:crit-findings}, \ref{fig:sev-score}, and \ref{fig:valid-findings}, we present the findings included in Table~\ref{table:perf} with confidence intervals. Each agent was given a single opportunity to find vulnerabilities in the target scope, and as a result we cannot present run-to-run variability. We compute 95\% confidence intervals for valid and critical findings using exact Poisson intervals, and we use bootstrap resampling to compute the confidence intervals on severity score. The Poisson assumption—that vulnerability discoveries follow an independent, constant-rate process—is imperfect here, and these intervals likely underestimate true uncertainty. For severity scores, we use bootstrap confidence intervals rather than Poisson methods because the metric is a weighted composite rather than a simple count; however, this approach conditions on the observed number of findings and captures only variability in severity composition, so it too should be interpreted as a lower bound on total uncertainty. Despite these limitations, ARTEMIS configurations, particularly $A_{2}$, far outperform the other evaluated agents. $A_{2}$'s lower confidence bound in terms of overall severity score exceeds the upper bound of all three non-ARTEMIS agent configurations, and nearly exceeds $A_{1}$'s as well. To ensure fairness with human participants—who could not reasonably be asked to repeat the engagement—we limited all participants to a single attempt. As mentioned in Section~\ref{sec:limitations}, a direction for future work is to create a runnable replica of the experiment's environment, in order to enable more thorough comparisons of AI agents.
\newpage
