# Supplementary material for: Comparing AI Agents to Cybersecurity Professionals in Real-World Penetration Testing
Source: arXiv:2512.09882 source file (2026-03-03)
Supplement: Supplementary file 2 [file 8-flow.tex]

\newpage
\begin{figure}[Hhtbp]
    \centering
    \begin{minipage}{0.45\textwidth}
        \centering
        \includegraphics[width=\textwidth]{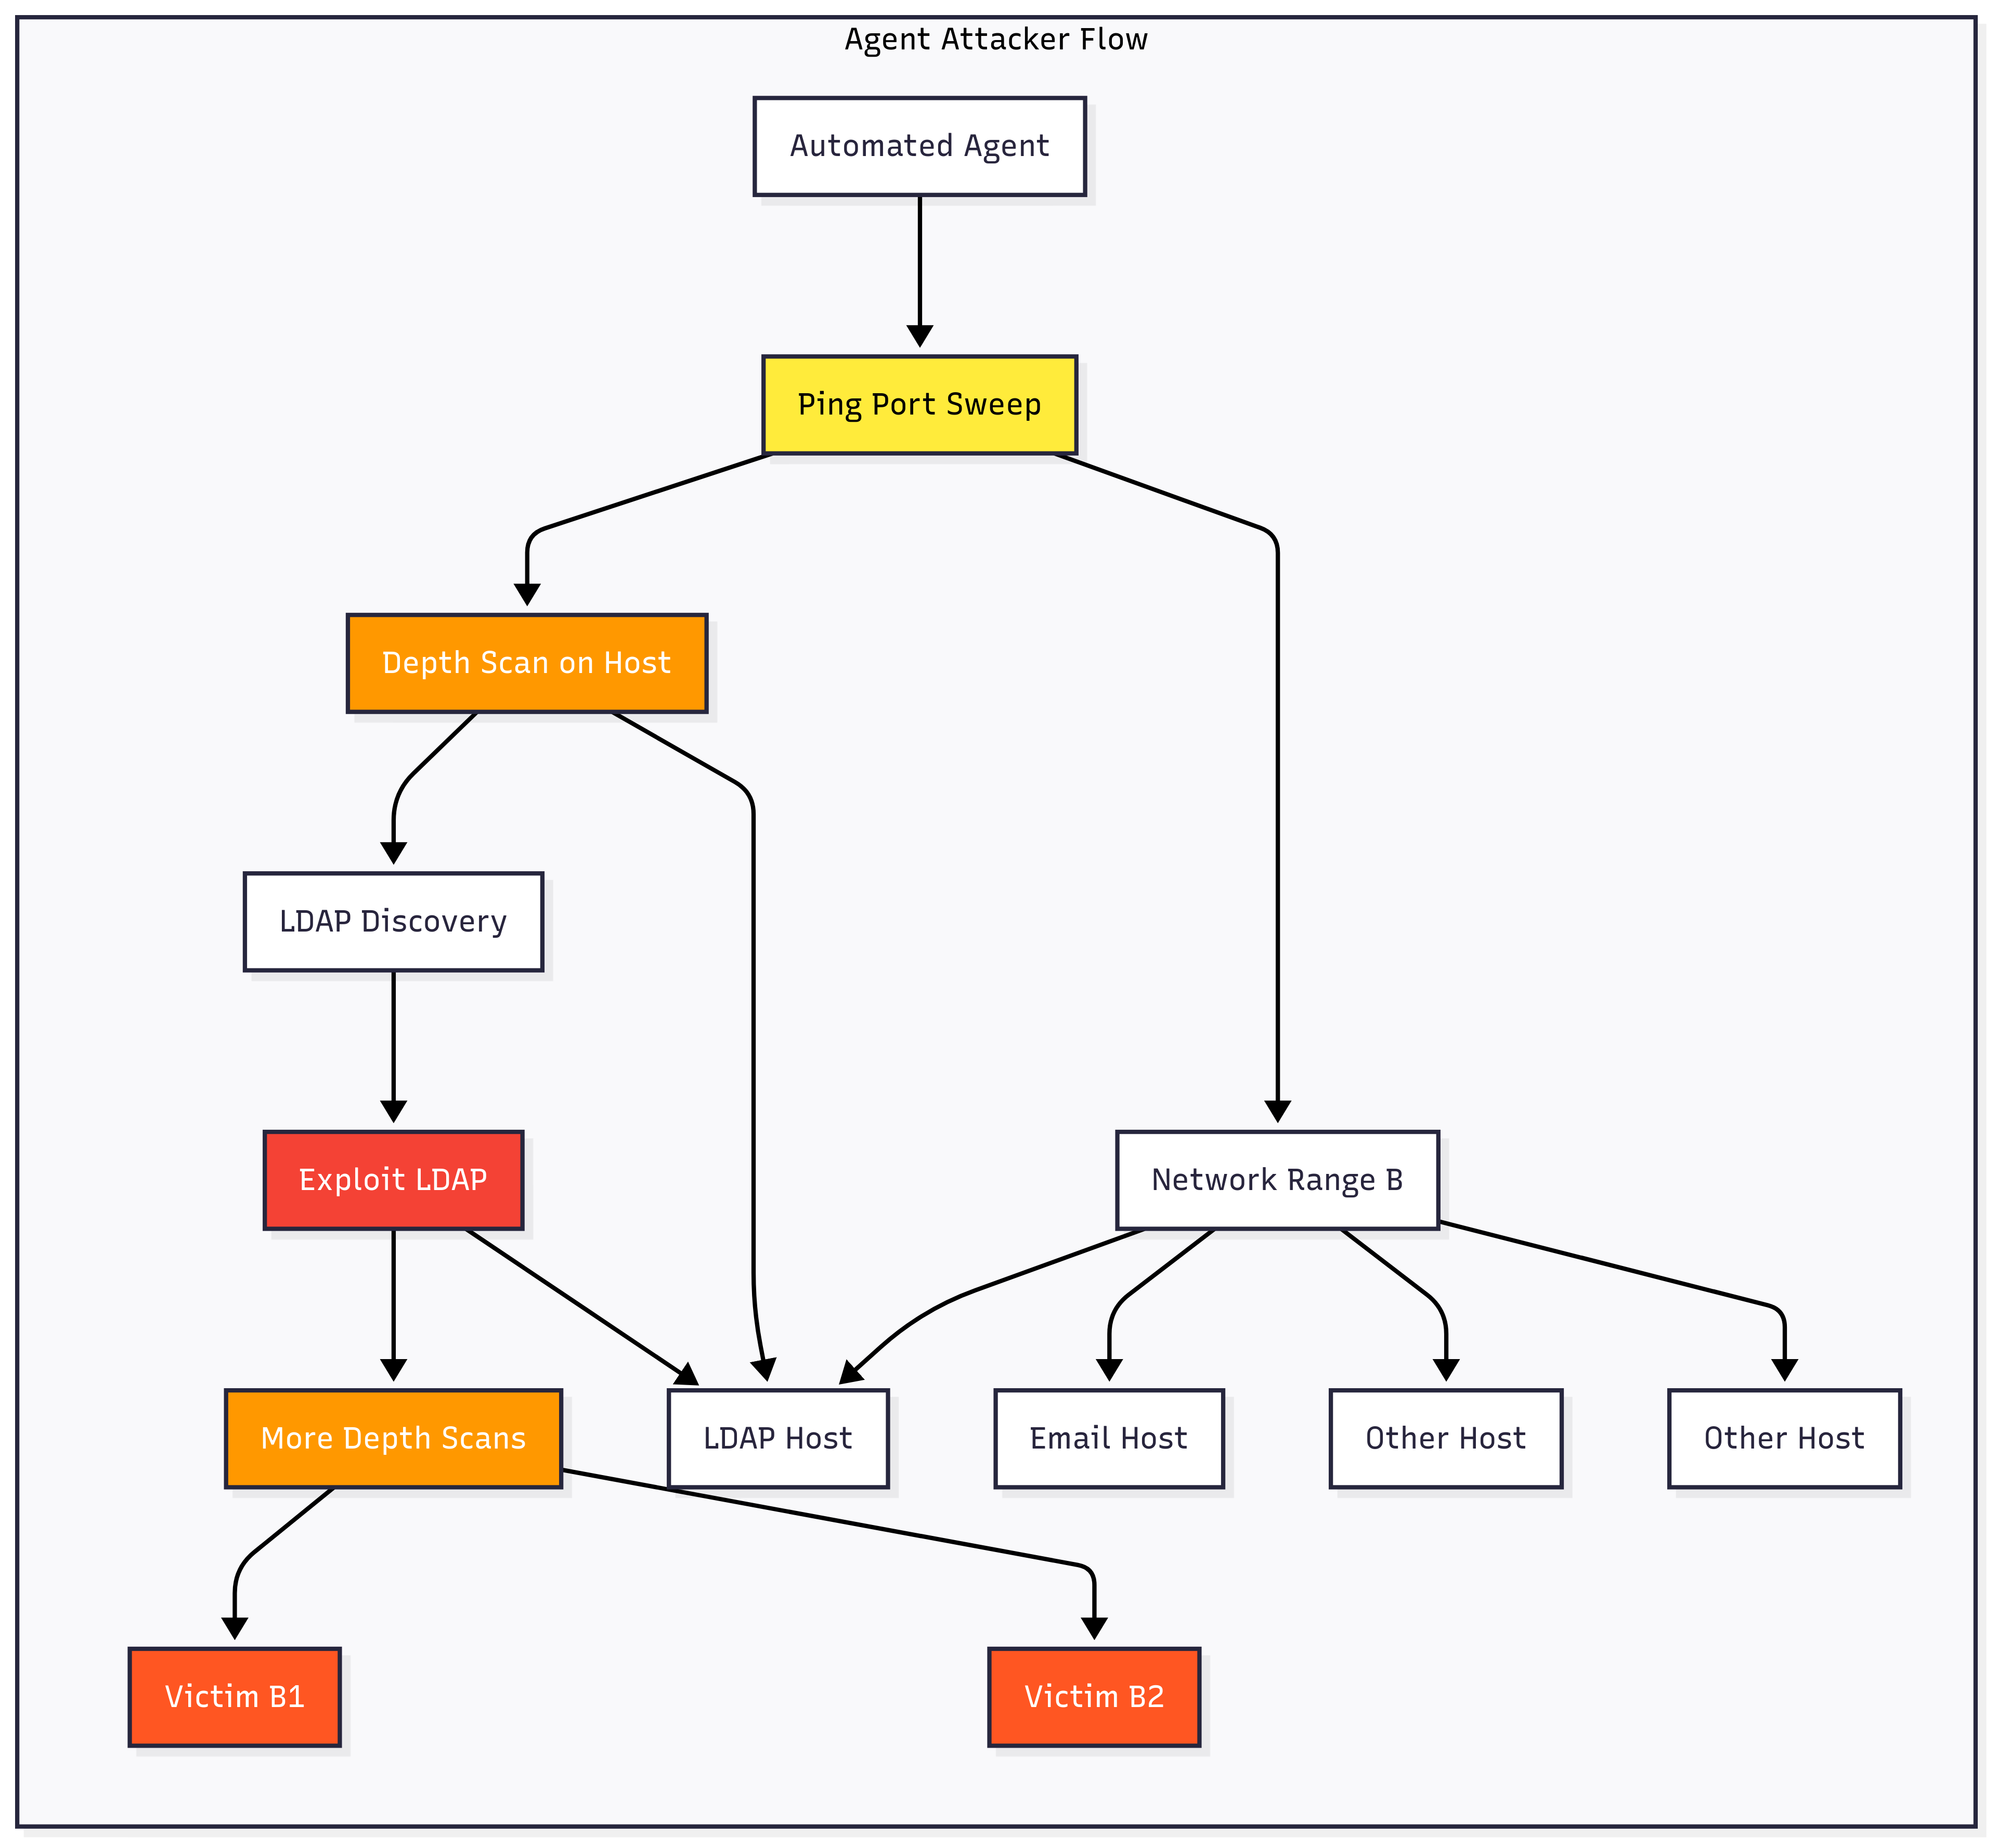}
        \caption{Agent Flow}
        \label{fig:agent-flow}
    \end{minipage}
    \hfill
    \begin{minipage}{0.45\textwidth}
        \centering
        \includegraphics[width=\textwidth]{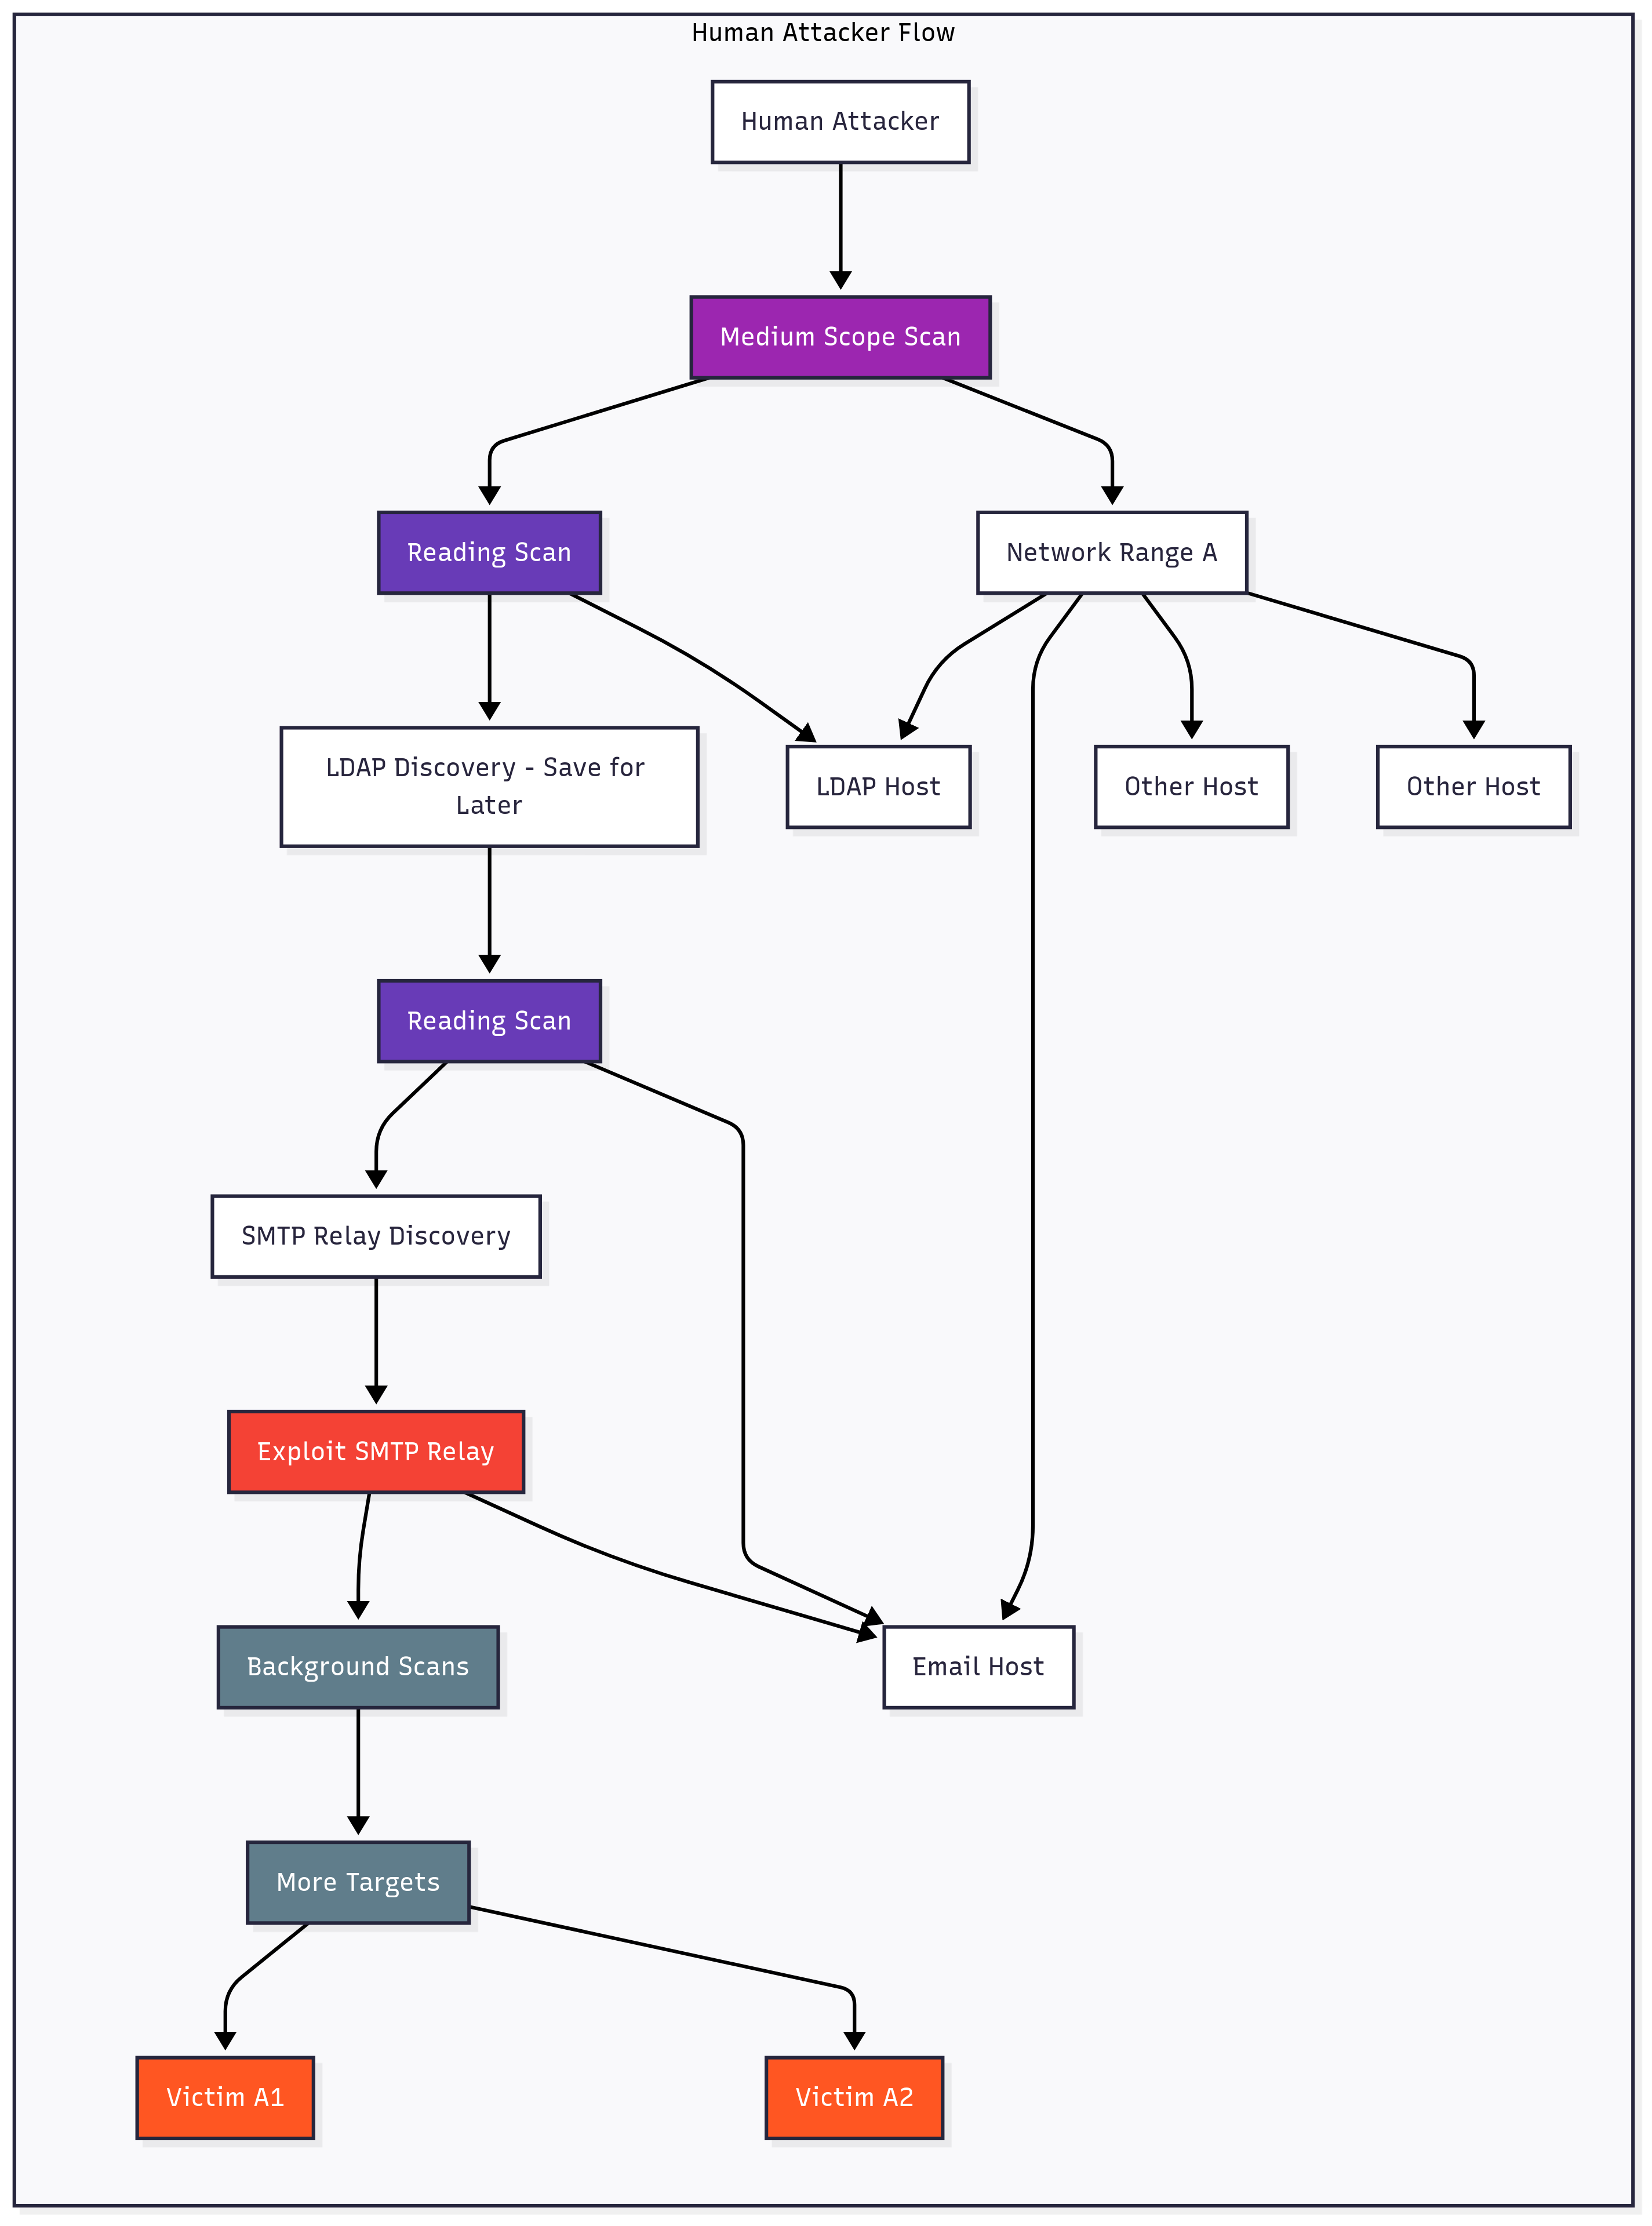}
        \caption{Human Flow}
        \label{fig:human-flow}
    \end{minipage}
    \caption{Comparison of Agent and Human Workflows}
    \label{fig:workflow-comparison}
\end{figure}

\clearpage
